# Supplementary material for: Isthmus: Bridging Supervision Islands Restores Uncertainty and Stability in One-Step Flows
Source: arXiv:2611.23616 source file (2026-11-17)
Supplement: Supplementary file 1 [file supp_labels.tex]

\makeatletter
\WarningFilter{hyperref}{Suppressing link with empty target}
\@namedef{r@S-cor:stability}{{S1}{6}{}{}{}}
\@namedef{r@S-cor:stability@cref}{{[spcorollary][1][]S1}{[1][6][]6}{}{}{}}
\@namedef{r@S-fig:direction}{{S10}{26}{}{}{}}
\@namedef{r@S-fig:direction@cref}{{[figure][10][]S10}{[1][25][]26}{}{}{}}
\@namedef{r@S-fig:heat}{{S8}{24}{}{}{}}
\@namedef{r@S-fig:heat@cref}{{[figure][8][]S8}{[1][22][]24}{}{}{}}
\@namedef{r@S-fig:mech-full}{{S5}{22}{}{}{}}
\@namedef{r@S-fig:mech-full@cref}{{[figure][5][]S5}{[1][21][]22}{}{}{}}
\@namedef{r@S-fig:share}{{S9}{24}{}{}{}}
\@namedef{r@S-fig:share@cref}{{[figure][9][]S9}{[1][24][]24}{}{}{}}
\@namedef{r@S-lem:fixedpoint}{{S1}{4}{}{}{}}
\@namedef{r@S-lem:fixedpoint@cref}{{[splemma][1][]S1}{[1][4][]4}{}{}{}}
\@namedef{r@S-prop:band}{{S3}{7}{}{}{}}
\@namedef{r@S-prop:band@cref}{{[spproposition][3][]S3}{[1][7][]7}{}{}{}}
\@namedef{r@S-prop:dyn}{{S5}{11}{}{}{}}
\@namedef{r@S-prop:dyn@cref}{{[spproposition][5][]S5}{[1][11][]11}{}{}{}}
\@namedef{r@S-prop:exact}{{S1}{5}{}{}{}}
\@namedef{r@S-prop:exact@cref}{{[spproposition][1][]S1}{[1][5][]5}{}{}{}}
\@namedef{r@S-prop:ident}{{S4}{8}{}{}{}}
\@namedef{r@S-prop:ident@cref}{{[spproposition][4][]S4}{[1][8][]8}{}{}{}}
\@namedef{r@S-prop:value}{{S2}{7}{}{}{}}
\@namedef{r@S-prop:value@cref}{{[spproposition][2][]S2}{[1][7][]7}{}{}{}}
\@namedef{r@S-rem:td}{{S1}{12}{}{}{}}
\@namedef{r@S-rem:td@cref}{{[remark][1][]S1}{[1][12][]12}{}{}{}}
\@namedef{r@S-sec:conventions}{{S1}{3}{}{}{}}
\@namedef{r@S-sec:conventions@cref}{{[section][1][]S1}{[1][3][]3}{}{}{}}
\@namedef{r@S-sec:distortion}{{S8}{19}{}{}{}}
\@namedef{r@S-sec:distortion@cref}{{[section][8][]S8}{[1][19][]19}{}{}{}}
\@namedef{r@S-sec:dyn}{{S11}{26}{}{}{}}
\@namedef{r@S-sec:dyn@cref}{{[section][11][]S11}{[1][26][]26}{}{}{}}
\@namedef{r@S-sec:eval}{{S7}{18}{}{}{}}
\@namedef{r@S-sec:eval@cref}{{[section][7][]S7}{[1][18][]18}{}{}{}}
\@namedef{r@S-sec:family}{{S5}{14}{}{}{}}
\@namedef{r@S-sec:family@cref}{{[section][5][]S5}{[1][14][]14}{}{}{}}
\@namedef{r@S-sec:impl}{{S6}{15}{}{}{}}
\@namedef{r@S-sec:impl@cref}{{[section][6][]S6}{[1][15][]15}{}{}{}}
\@namedef{r@S-sec:lg}{{S3}{13}{}{}{}}
\@namedef{r@S-sec:lg@cref}{{[section][3][]S3}{[1][13][]13}{}{}{}}
\@namedef{r@S-sec:mri}{{S9}{20}{}{}{}}
\@namedef{r@S-sec:mri@cref}{{[section][9][]S9}{[1][20][]20}{}{}{}}
\@namedef{r@S-sec:proofs}{{S2}{3}{}{}{}}
\@namedef{r@S-sec:proofs@cref}{{[section][2][]S2}{[1][3][]3}{}{}{}}
\@namedef{r@S-sec:related-ext}{{S14}{34}{}{}{}}
\@namedef{r@S-sec:related-ext@cref}{{[section][14][]S14}{[1][34][]34}{}{}{}}
\@namedef{r@S-tab:family}{{S2}{16}{}{}{}}
\@namedef{r@S-tab:family@cref}{{[table][2][]S2}{[1][15][]16}{}{}{}}
\@namedef{r@S-tab:fastmri}{{S16}{30}{}{}{}}
\@namedef{r@S-tab:fastmri@cref}{{[table][16][]S16}{[1][29][]30}{}{}{}}
\@namedef{r@S-tab:long}{{S12}{27}{}{}{}}
\@namedef{r@S-tab:long@cref}{{[table][12][]S12}{[1][27][]27}{}{}{}}
\@namedef{r@S-tab:mri-full}{{S7}{21}{}{}{}}
\@namedef{r@S-tab:mri-full@cref}{{[table][7][]S7}{[1][20][]21}{}{}{}}
\@namedef{r@S-tab:snap-ixi}{{S10}{25}{}{}{}}
\@namedef{r@S-tab:snap-ixi@cref}{{[table][10][]S10}{[1][25][]25}{}{}{}}
\@namedef{r@S-tab:uncond-seeds}{{S18}{30}{}{}{}}
\@namedef{r@S-tab:uncond-seeds@cref}{{[table][18][]S18}{[1][30][]30}{}{}{}}
\makeatother
